# Supplementary material for: FORAY: Towards Effective Attack Synthesis against Deep Logical Vulnerabilities in DeFi Protocols
Source: arXiv:2407.06348 source file (2024-11-20)
Supplement: Supplementary file 1 [file appendix.tex]

\section{Appendix}
\label{apdx}

\begin{table*}[t!]
    \centering
    \caption{Compare \tool against \halmos and \ityfuzz.}
    % \footnotesize
    \begin{tabular}{|c|l|c|c|c|c|}
        \hline 
         Name & Category & \tool & \ityfuzz & \halmos & Loss (USD) \\ \hline
         AES  & Token Burn & 25.0s & 27.0s & TO & 60K \\ \hline 
         BGLD & Token Burn & 24.6s & 172.0s & TO & 18K \\ \hline 
         BIGFI & Token Burn & 25.5s & 511.0s & TO & 30K \\ \hline
         BXH & Pump\&Dump & 27.0s & TO & TO & 40K \\ \hline
         Discover & Price Discrepancy & 25.8s & NA & 10251.3s & 15K \\ \hline
         % 5
         EGD & Pump\&Dump & 327.3s & 2.0s & TO & 36K \\ \hline
         MUMUG & Price Discrepancy & 325.6s & NA & 7681.7s & 57K \\ \hline
         NOVO & Token Burn & 24.8s & 81.0s & TO & 85K \\ \hline
         OneRing & Pump\&Dump & 26.8s & TO & TO & 1.5M \\ \hline
         RADTDAO & Token Burn & 24.7s & 627.0s & TO & 94K \\ \hline
         % 10
         RES & Swap Rate Manipulate & 25.7s & 3.0s & TO & 290K \\ \hline
         SGZ & Swap Rate Manipulate & 25.6s & TO & TO & 25K \\ \hline
         ShadowFi & Token Burn & 25.8s & 1757.0s & TO & 330K \\ \hline
         Zoompro & Swap Rate Manipulate & 28.8s & TO & TO & 61K \\ \hline
         NXUSD & Pump\&Dump & 626.3s & TO & TO & 50K \\ \hline
         % 15
         NMB & Pump\&Dump & TO & TO & TO & 76K \\ \hline
         Lodestar & Pump\&Dump & TO & TO & TO & 4.0M \\ \hline
         SafeMoon & Token Burn & 27.8s & TO & TO & 8.9M \\ \hline
         Allbridge & Price Discrepancy & TO & NA & TO & 550K \\ \hline
         Swapos V2 & Swap Rate Manipulate & 26.1s & 321.0s & 6322.0s & 468K \\ \hline
         % 20
         Axioma & Pump\&Dump & 24.1s & 123.0s & TO & 5K \\ \hline
         0vix & Price Discrepancy & TO & NA & TO & 2M \\ \hline
         NeverFall & Pump\&Dump & 24.8s & TO & TO & 74K \\ \hline
         SellToken02 & Pump\&Dump & 623.2s & TO & TO & 197K \\ \hline
         LW & Price Discrepancy & 1225.5s & NA & TO & 50K \\ \hline
         % 25
         ERC20TokenBank & Pimp\&Pump & 619.7s & TO & TO & 111K \\ \hline
         UN & Token Burn & 25.3s & 10.1s & TO & 26K \\ \hline
         CFC & Token Burn & 326.1s & 164.0s & TO & 16K \\ \hline
         Themis & Pump\&Dump & TO & TO & TO & 370K \\ \hline
         Bamboo & Token Burn & 341.3s & 42.0s & TO & 50K \\ \hline
         % 30
         LUSD & Pump\&Dump & 1250.1s & TO & TO & 10K \\ \hline
         RodeoFinance & Price Discrepancy & TO & NA & TO & 888K \\ \hline
         Conic & Pump\&Dump & 618.7s & TO & TO & 934K \\ \hline
         Carson & Price Discrepancy & TO & TO & TO & 150K \\ \hline
         & Avg. Time &  249.0s & 295.4s & 8085.0s & Sum: 21.6M \\ \hline
    \end{tabular}
    \label{tab:comp-full}
\end{table*}
